# Supplementary material for: Uncertainty-Guided Self-Questioning and Answering for Video-Language Alignment
Source: arXiv:2410.02768 source file (2025-05-06)
Supplement: Supplementary file 1 [file appendix-llama3.1.tex]

\begin{table*}[h]
\label{table1}
    \centering
    \begin{adjustbox}{width=0.99\textwidth}
    \begin{tabular}{c|c|c c c c >{\columncolor{lightgreen}} c| >{\columncolor{lightgreen}}c|>{\columncolor{lightgreen}} c| >{\columncolor{lightgreen}}c| >{\columncolor{lightgreen}}c }
        \toprule
         \multirow{2}{*}{\textbf{Language Model}} & \multirow{2}{*}{\shortstack{\textbf{\# trainable} \\ \textbf{params}}}  & \multicolumn{5}{c|}{\textbf{STAR}} & \multicolumn{1}{c|}{\textbf{DramaQA}} & \multicolumn{1}{c|}{\textbf{VLEP}} & \multicolumn{1}{c|}{\textbf{TVQA*}} & \multicolumn{1}{c}{\textbf{How2QA}} \\ 
        &  & Int. & Seq. & Pre. & Fea. & Tot. & Tot. & Tot. & Tot. & Tot. \\
        \midrule

        \multicolumn{1}{l|}{LLaMA1-7B} & \textbf{4.5M}  & 66.9 & 68.0 & 62.0 & 57.2 & 66.4 & \textbf{85.2} & \textbf{71.2} &  \textbf{71.6} & 89.4 \\
        \multicolumn{1}{l|}{LLaMA3.1-8B} &  \textbf{4.5M}  & 66.9 & 68.0 & 62.0 & 57.2 & 66.4 & \textbf{85.5} & \textbf{71.2} &  \textbf{71.6} & 89.4 \\
        
        \bottomrule
    \end{tabular}
    \end{adjustbox}
    \caption{\textbf{Comparison on five challenging VideoQA benchmarks with LLaMA1-7B and LLaMA3.1-8B.} * denotes that we do not use the speech captions.
    }
    \label{tab:main}
\end{table*}
